# Supplementary material for: YOLO-RD: Introducing Relevant and Compact Explicit Knowledge to YOLO by Retriever-Dictionary
Source: arXiv:2410.15346 source file (2025-02-08)
Supplement: Supplementary file 1 [file estimate.tex]

\begin{figure}
    \centering
    \begin{subfigure}[b]{0.48\linewidth}
        \includegraphics[width=\textwidth]{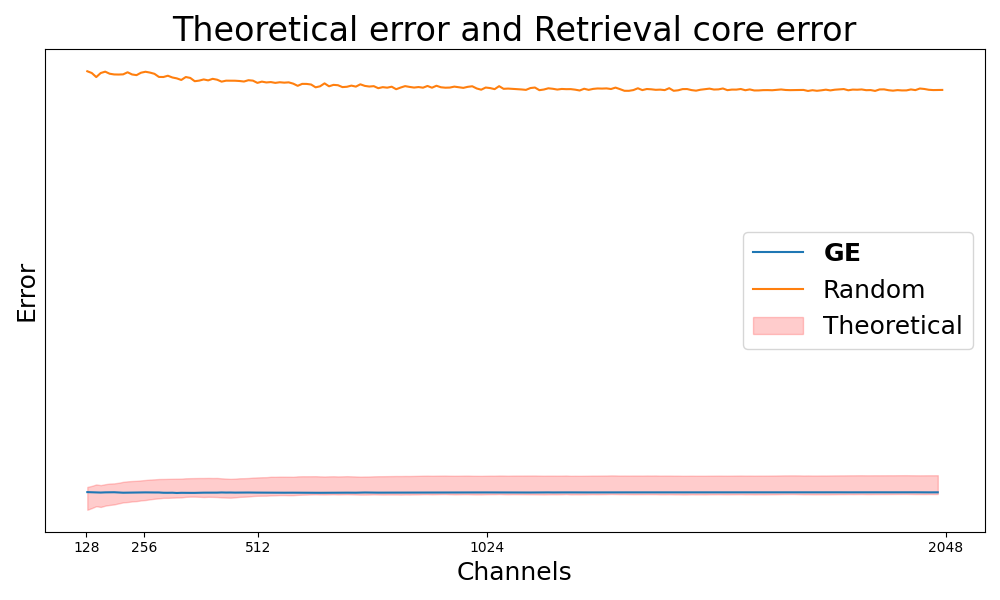}
    \end{subfigure}
    \hfill
    \begin{subfigure}[b]{0.48\linewidth}
        \includegraphics[width=\textwidth]{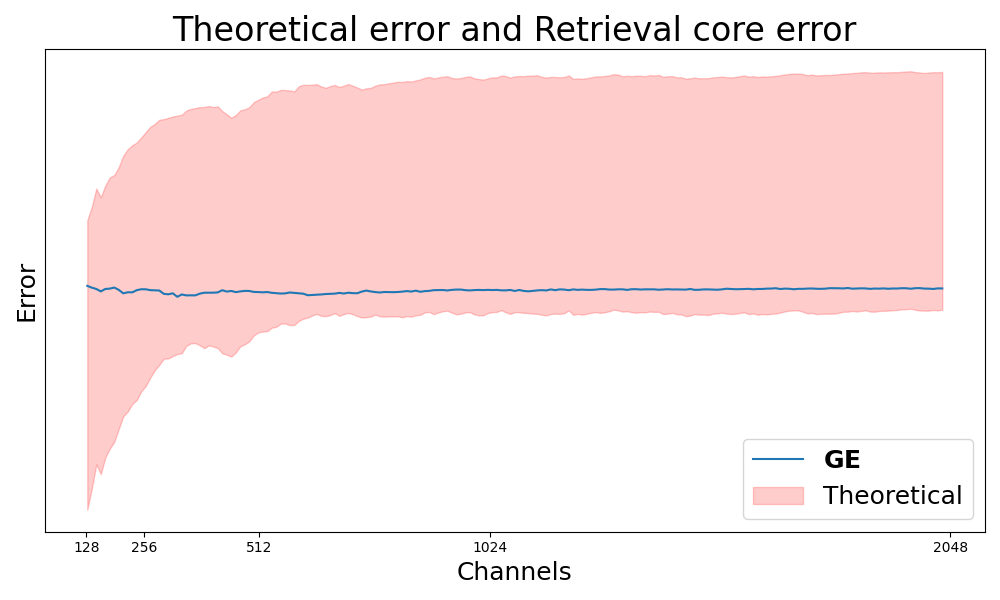}
    \end{subfigure}
    \caption{The error of Random, Theoretical, and $\mathbf{GE}$ between $W_{eq}$}
    \label{fig: estimate_error}
\end{figure}
