# Supplementary material for: YOLO-RD: Introducing Relevant and Compact Explicit Knowledge to YOLO by Retriever-Dictionary
Source: arXiv:2410.15346 source file (2025-02-08)
Supplement: Supplementary file 2 [file more_vis.tex]

\begin{figure}
    \centering
    \begin{tabular}{cccccc}
        \toprule
        \textbf{input} & \textbf{without RD} & \textbf{with RD} & \textbf{input} & \textbf{without RD} & \textbf{with RD} \\
        \midrule
        \includegraphics[width=0.15\textwidth]{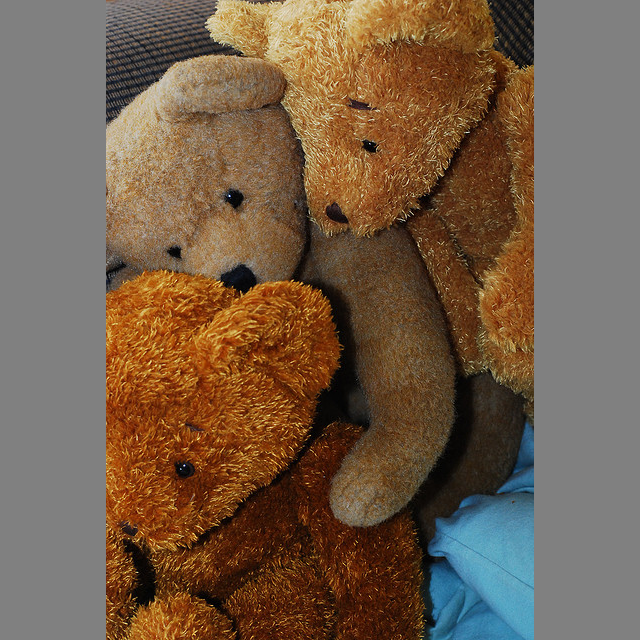} & \includegraphics[width=0.15\textwidth]{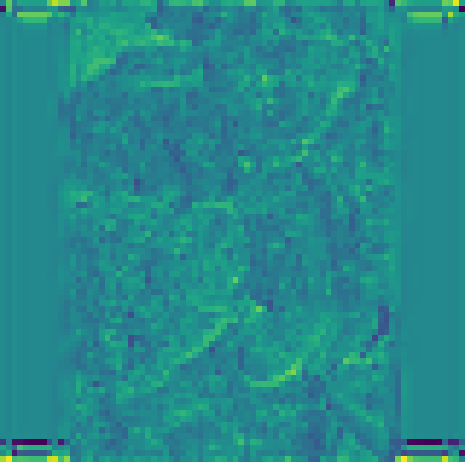} & \includegraphics[width=0.15\textwidth]{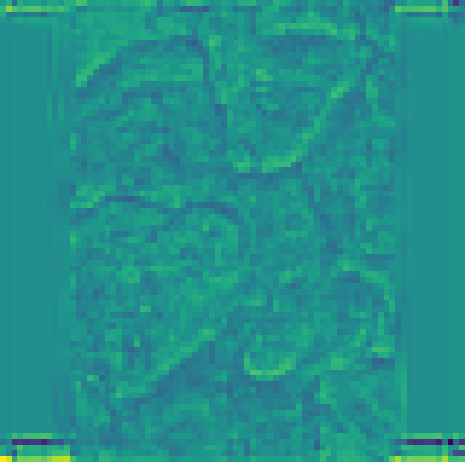} & 
        
        \includegraphics[width=0.15\textwidth]{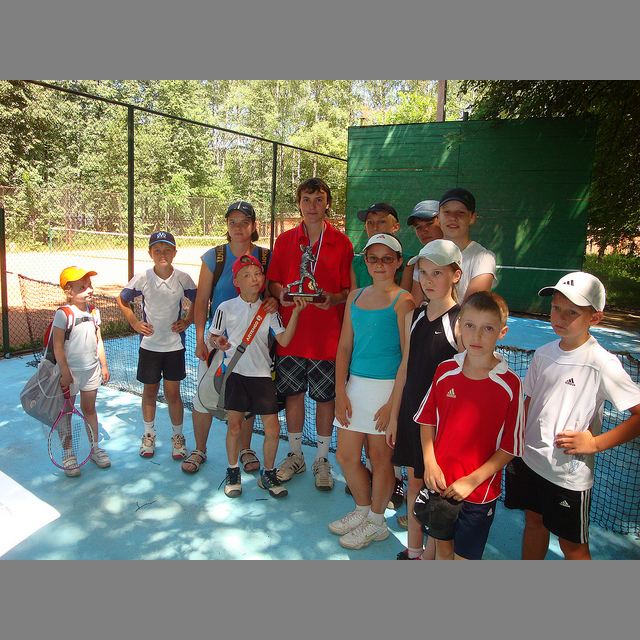} & \includegraphics[width=0.15\textwidth]{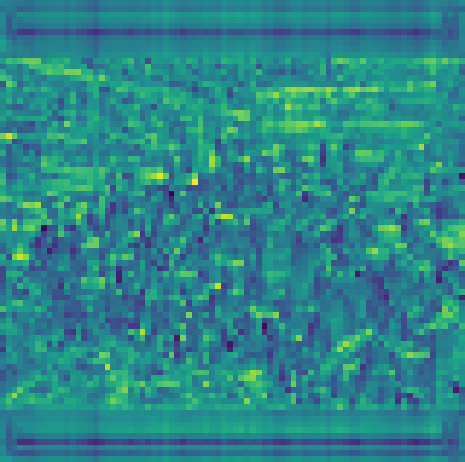} & 
        \includegraphics[width=0.15\textwidth]{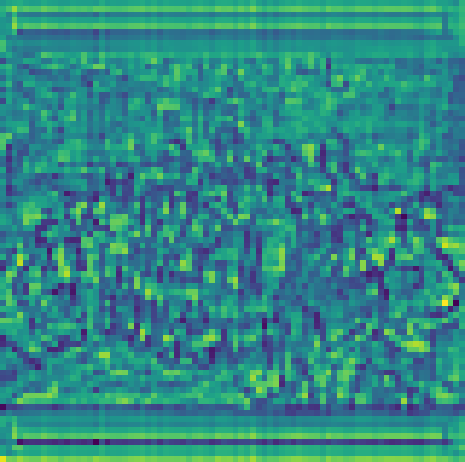}  \\
        
        \includegraphics[width=0.15\textwidth]{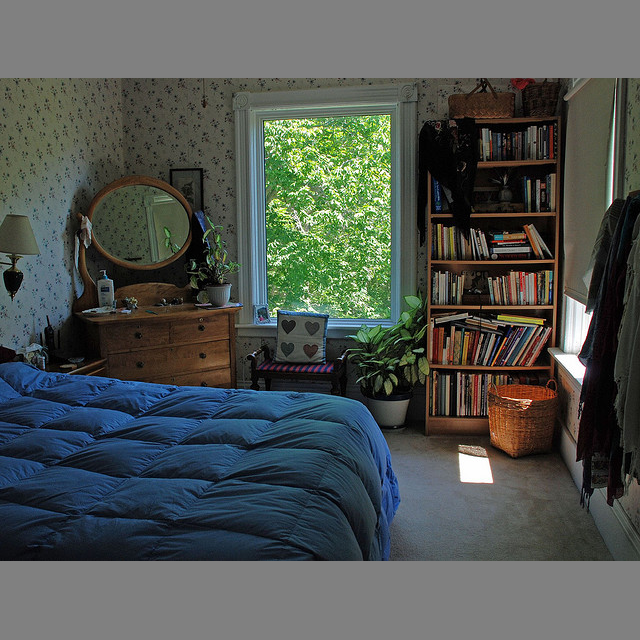} & \includegraphics[width=0.15\textwidth]{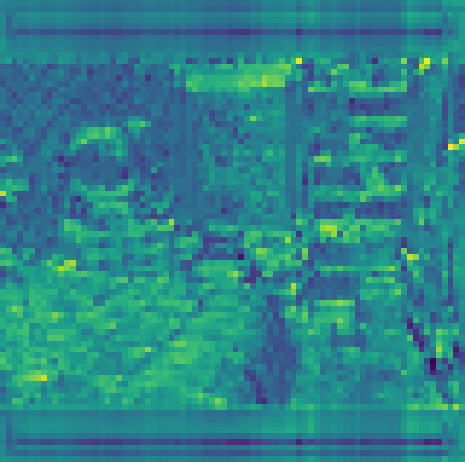} & \includegraphics[width=0.15\textwidth]{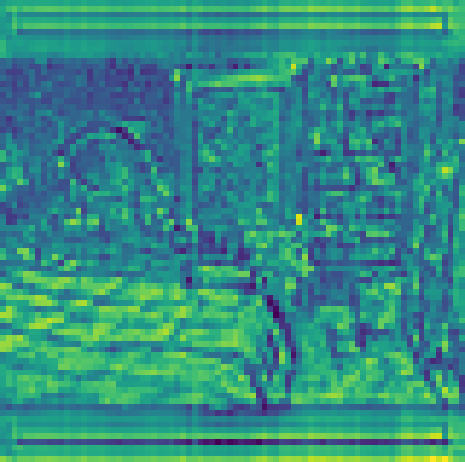} & 
        
        \includegraphics[width=0.15\textwidth]{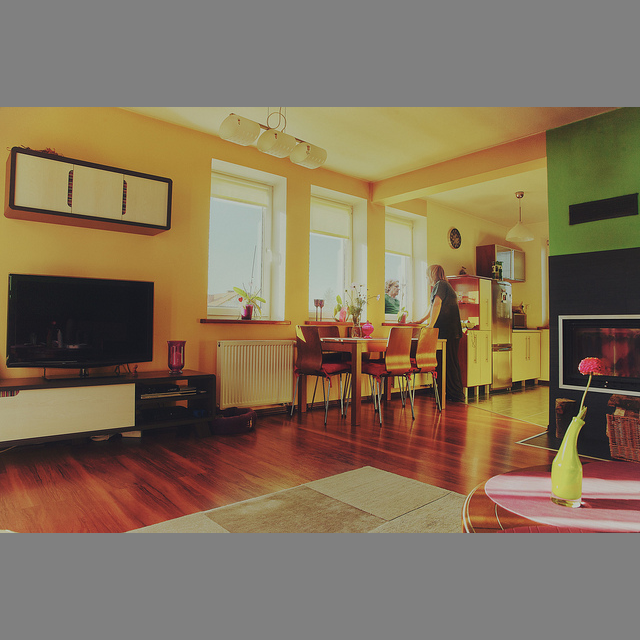} & \includegraphics[width=0.15\textwidth]{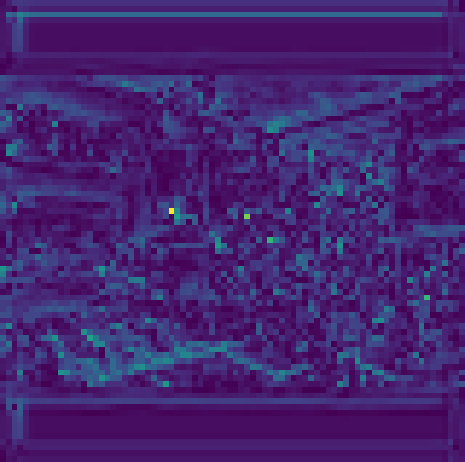} & \includegraphics[width=0.15\textwidth]{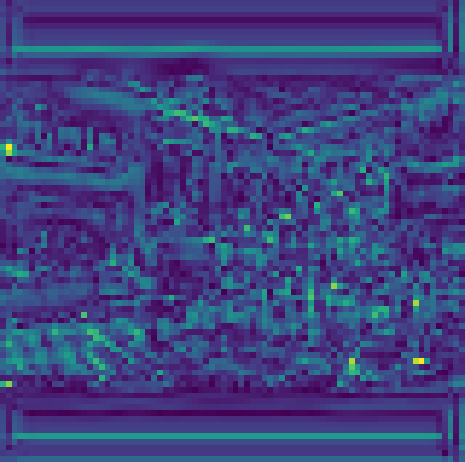} \\
        
        \includegraphics[width=0.15\textwidth]{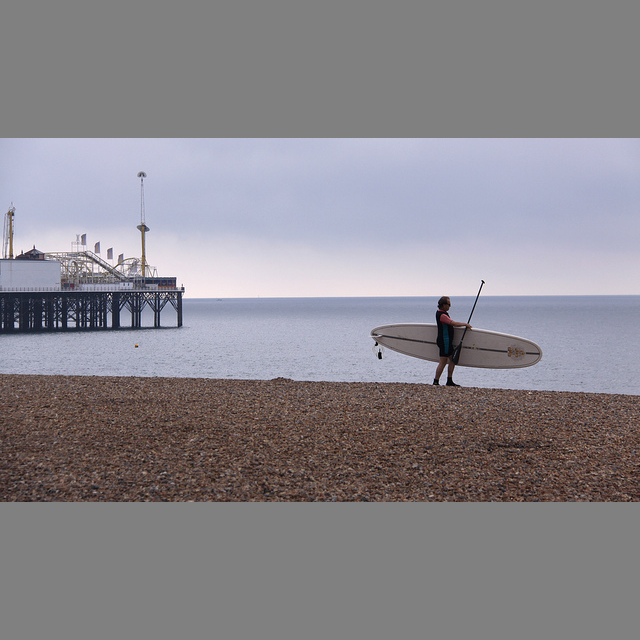} & \includegraphics[width=0.15\textwidth]{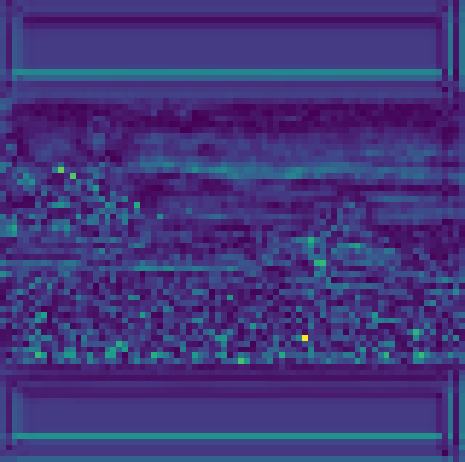} & \includegraphics[width=0.15\textwidth]{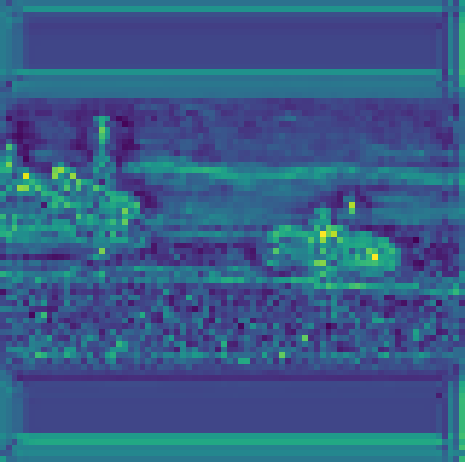} & 
        
        \includegraphics[width=0.15\textwidth]{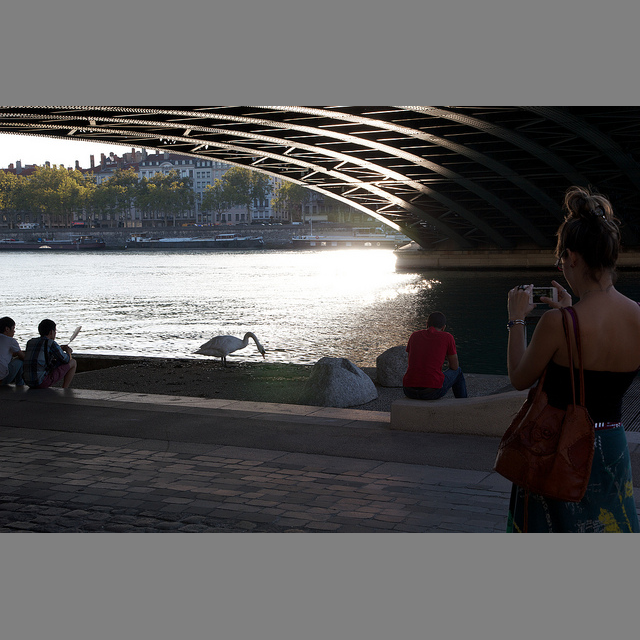} & \includegraphics[width=0.15\textwidth]{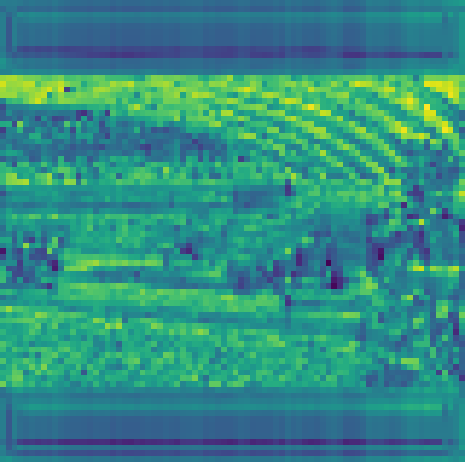} & \includegraphics[width=0.15\textwidth]{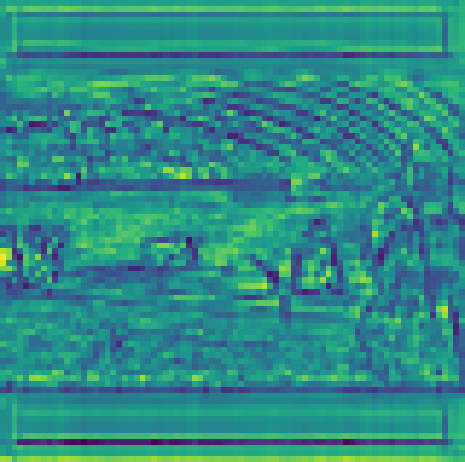}  \\
        \bottomrule
    \end{tabular}
    \caption{More visualization of RD}
    \label{fig: woRDmore}
\end{figure}
\begin{figure}
    \centering
    \begin{tabular}{cccccc}
        \toprule
        \textbf{Ground Truth} & \textbf{without RD} & \textbf{with RD} & \textbf{Ground Truth} & \textbf{without RD} & \textbf{with RD} \\
        \midrule
        \includegraphics[width=0.15\textwidth]{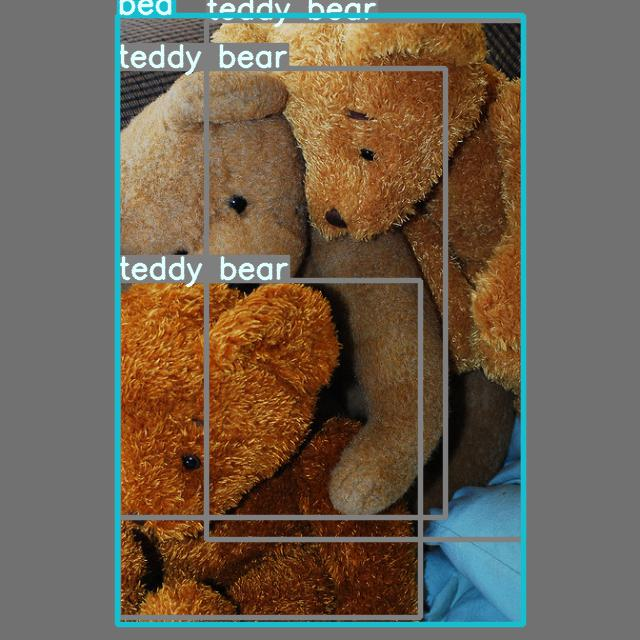} & \includegraphics[width=0.15\textwidth]{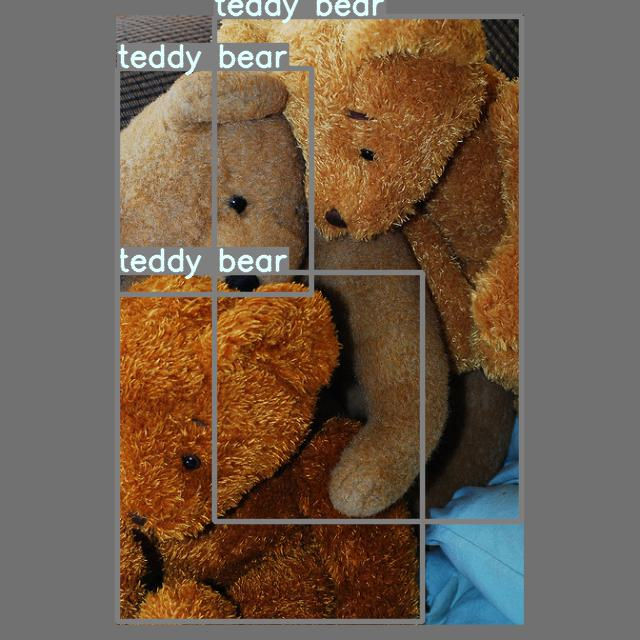} & \includegraphics[width=0.15\textwidth]{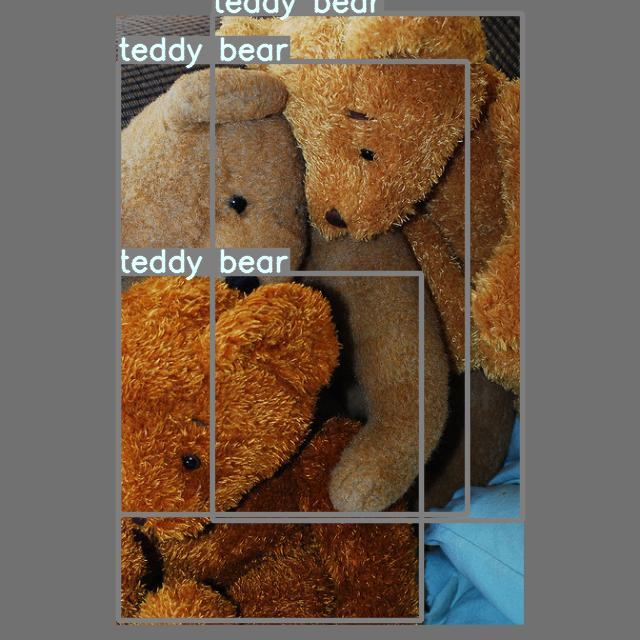} & 
        
        \includegraphics[width=0.15\textwidth]{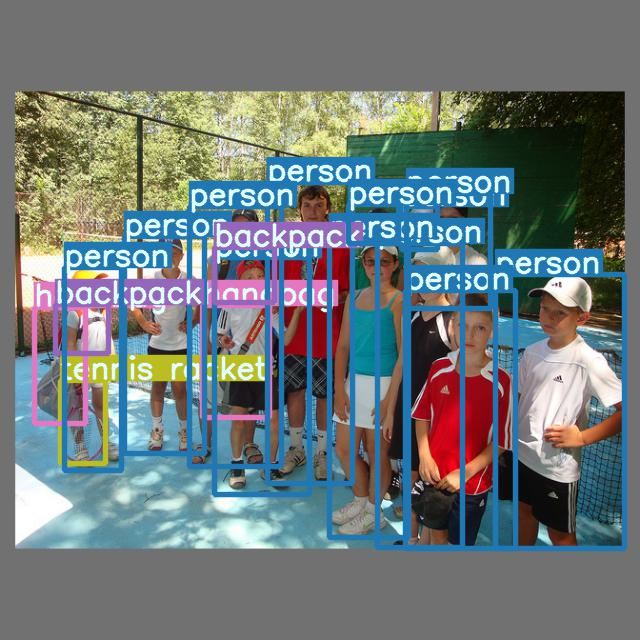} & \includegraphics[width=0.15\textwidth]{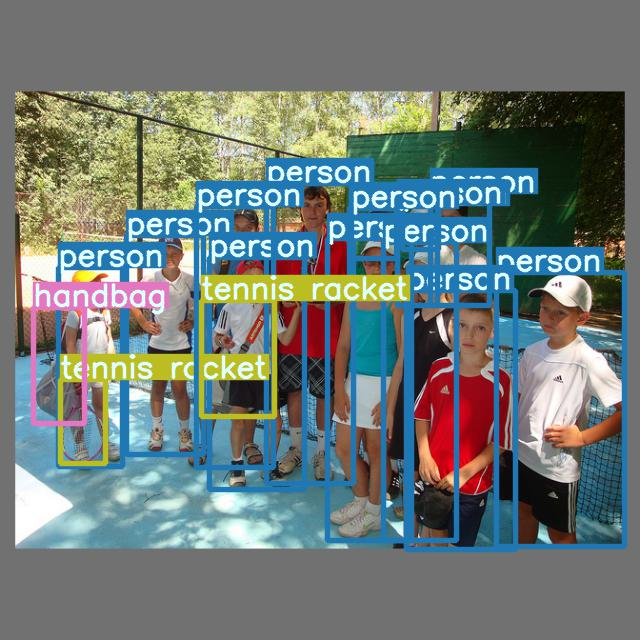} & 
        \includegraphics[width=0.15\textwidth]{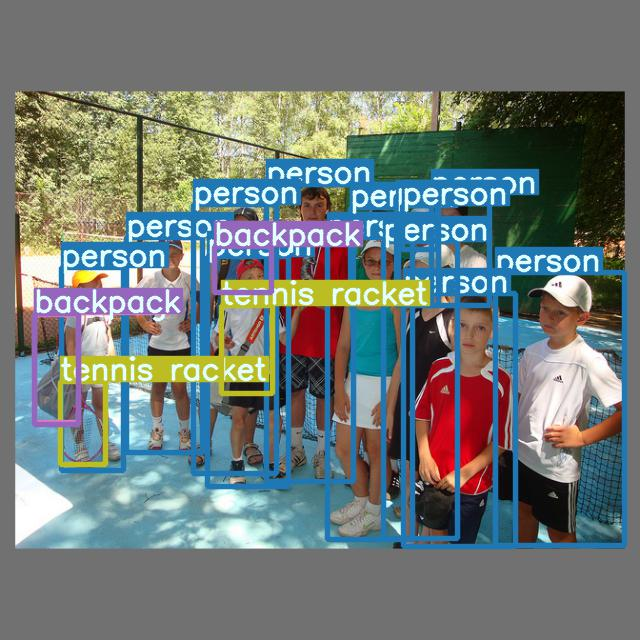}  \\
        
        \includegraphics[width=0.15\textwidth]{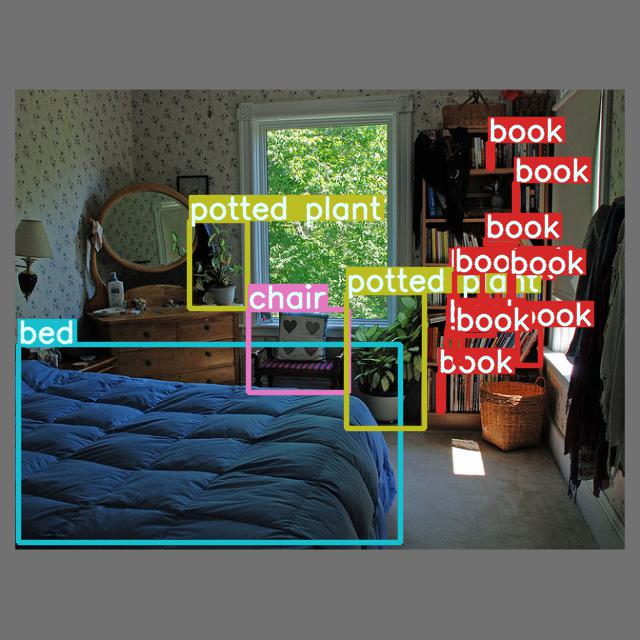} & \includegraphics[width=0.15\textwidth]{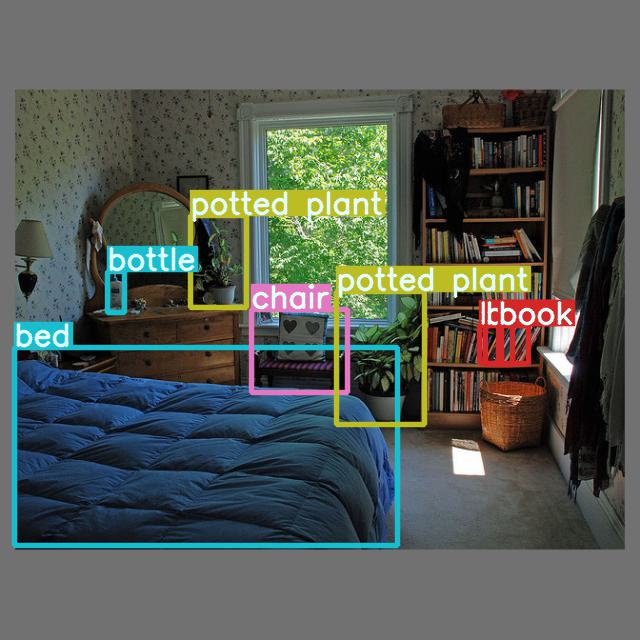} & \includegraphics[width=0.15\textwidth]{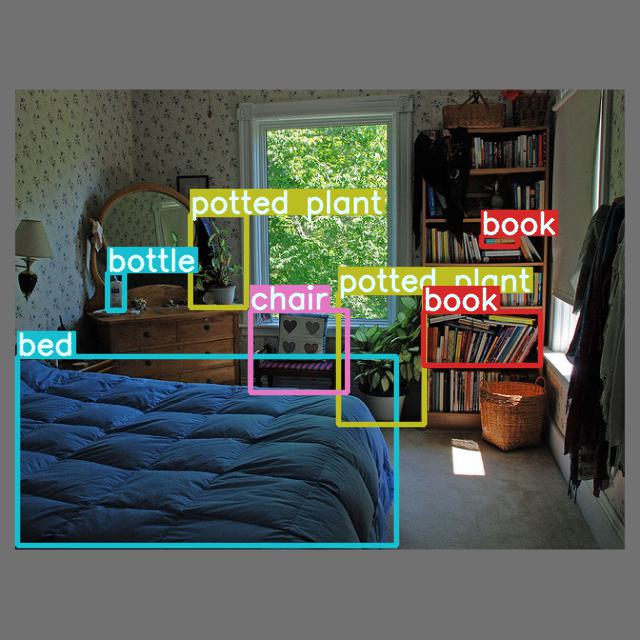} & 
        
        \includegraphics[width=0.15\textwidth]{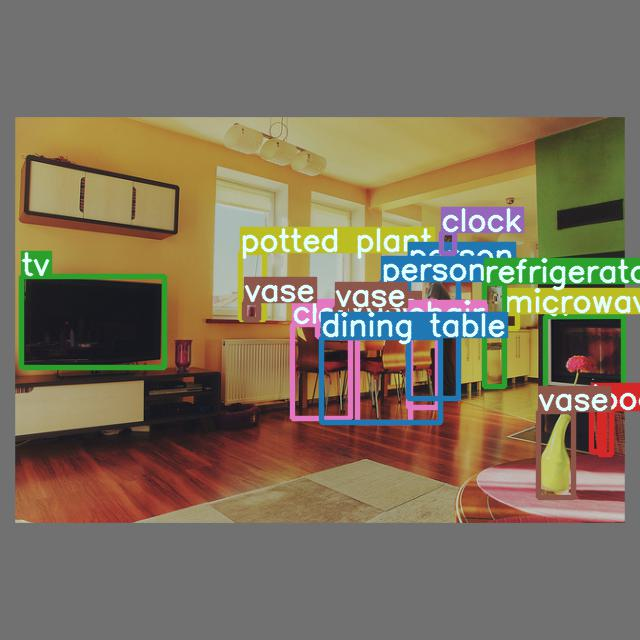} & \includegraphics[width=0.15\textwidth]{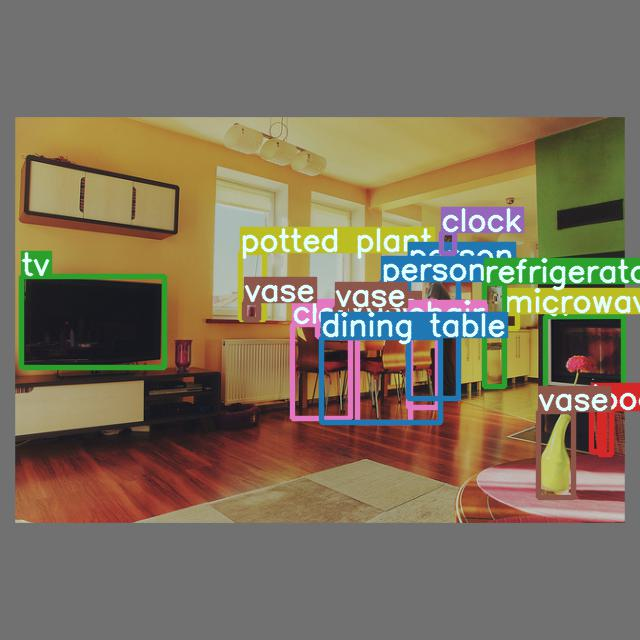} & \includegraphics[width=0.15\textwidth]{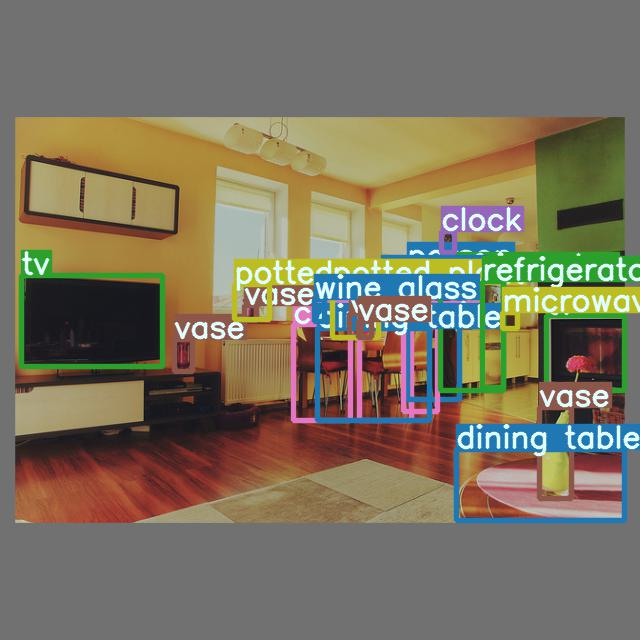} \\
        
        \includegraphics[width=0.15\textwidth]{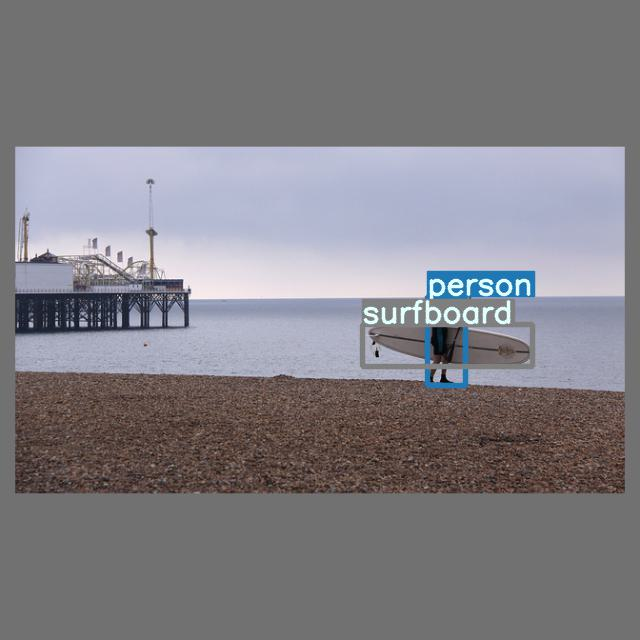} & \includegraphics[width=0.15\textwidth]{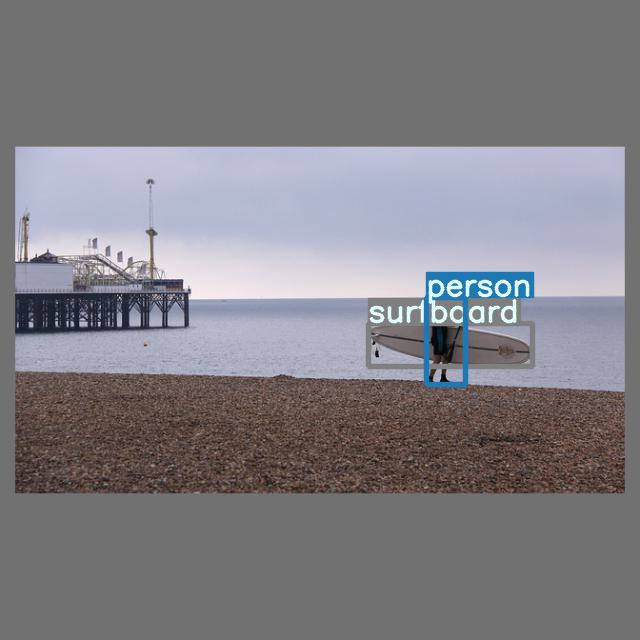} & \includegraphics[width=0.15\textwidth]{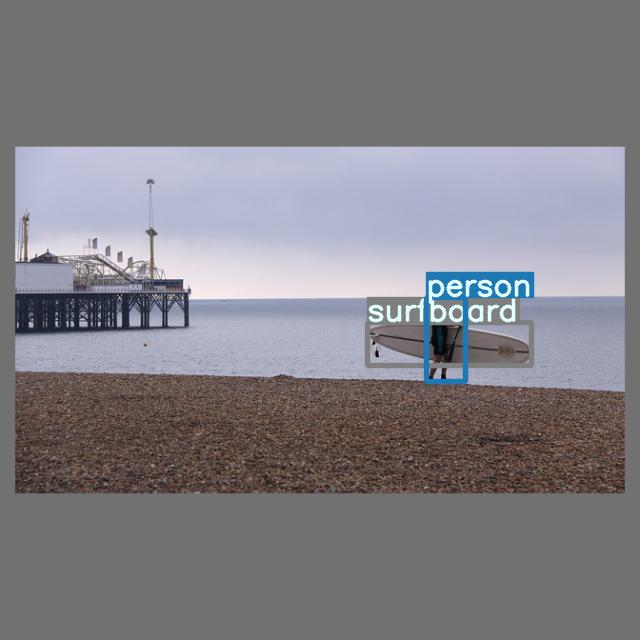} & 
        
        \includegraphics[width=0.15\textwidth]{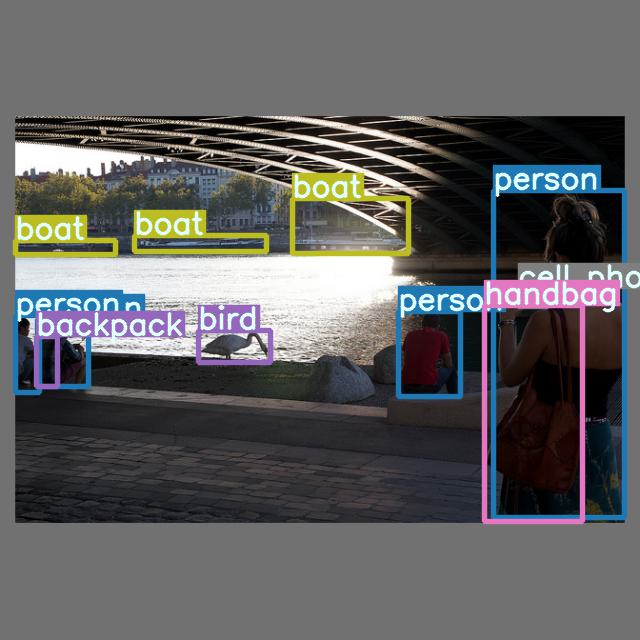} & \includegraphics[width=0.15\textwidth]{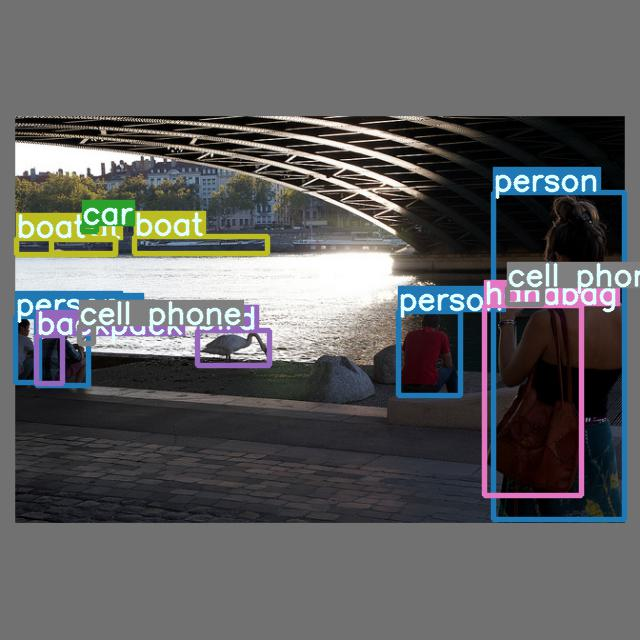} & \includegraphics[width=0.15\textwidth]{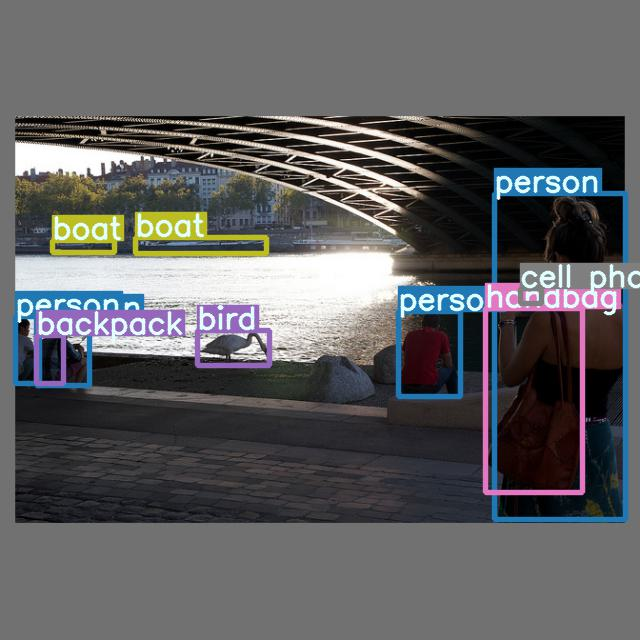}  \\
        \bottomrule
    \end{tabular}
    \caption{More visualization of RD}
    \label{fig: woRDres}
\end{figure}
